# Supplementary material for: Lifting topological codes: Three-dimensional subsystem codes from two-dimensional anyon models
Source: arXiv:2305.06365 source file (2024-05-18)

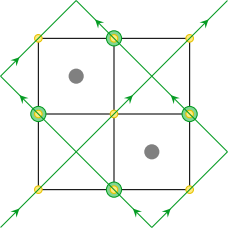

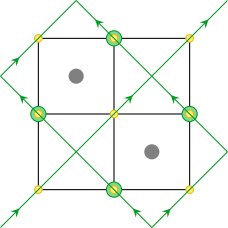

Supplement: Supplementary file 1 [file topFaceAdditional.pdf]
